# Supplementary material for: Learning Markovian Dynamics with Spectral Maps
Source: arXiv:2311.16411 ancillary file (2024-09-25)
Supplement: Supplementary file 1 [file sm.pdf]

# Learning Markovian Dynamics with Spectral Maps

*Supplementary Material*

Jakub Rydzewski[a] and Tuğçe Gökdemir

*Institute of Physics, Faculty of Physics, Astronomy and Informatics, Nicolaus Copernicus University, Grudziadzka 5, 87-100 Toruń, Poland*

(Dated: 28 November 2023)

## S1. Simulation Datasets

### 1. Müller–Brown Potential

Following Ref. 1, we defina a three-state Müller–Brown potential as:

$$F(x_1, x_2) = B \sum_k A_k \, \mathrm{e}^{p_k(x_1,x_2)} + F_0, \tag{S1}$$

where the exponent $p(x_1, x_2)$ is a polynomial:

$$\begin{aligned} p_k(x_1, x_2) = &\, a_k(x_1 - x_k)^2 \\ &+ b_k(x_1 - x_k)(x_2 - y_k) \\ &+ c_k(x_2 - y_k)^2. \end{aligned} \tag{S2}$$

The parameters in Eq. S1 and Eq. S2 are:

| $A_k$ | $a_k$ | $b_k$ | $c_k$ | $x$ | $y$ |
|---|---|---|---|---|---|
| -280 | -15 | 0 | -10 | 1 | 0 |
| -170 | -1 | 0 | -10 | 0.2 | 0.5 |
| -170 | -6.5 | 11 | -6.5 | -0.5 | 1.5 |
| 15 | 0.7 | 0.6 | 0.7 | -1 | 1 |

with the barrier parameter $B = 0.15\ k_\mathrm{B}T$ and the shift $F_0 = 146.7\ k_\mathrm{B}T$.

### 2. CLN025

Molecular dynamics simulations of CLN025 are obtained from D.E. Shaw Research.[2] For detailed simulation protocols, see Ref. 2 and its corresponding Supporting Online Material. The trajectory of ∼100-$\mu$s in the NVT ensemble at a temperature of 340 K with conformations recorded every 200 ps is used. As a high-dimensional representation, pairwise Euclidean distances between the C$\alpha$ atoms of CLN are employed, which amounts to $n = 45$ configuration variables. The training set consists of 10000 high-dimensional samples (extracted from the simulation every 1 ns) with a batch size of 2000 samples. Spectral map is used to construct CVs for $k = 2$ metastable states.

## S2. Implementation

The code for spectral map is implemented using PyTorch.[3] The Markov state model analysis is performed using PyEmma.[4]

[a] jr@fizyka.umk.pl

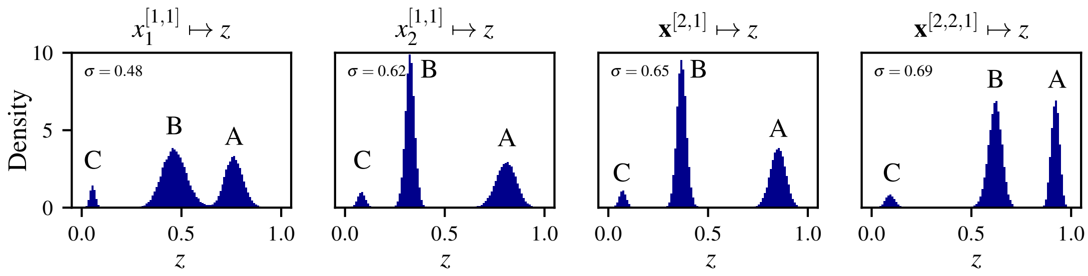


FIG. S1. Training the target mapping $\xi_w(\mathbf{x}) = \mathbf{z}$ on the three-state Müller–Brown potential (A, B, C). Densities along the $z$ variable for different architectures, e.g., $\mathbf{x}^{[a,b]} \mapsto z$ denotes mapping the $\mathbf{x}$ variable through a network consisting of $[a, b]$ layers to the $z$ CV. Spectral gap values $\sigma$ are given in the top-left corner. The following variables are used as CVs: the $x_1$ variable, the $x_2$ variable, a linear combination of $x_1$ and $x_2$, a nonlinear combination of $x_1$ and $x_2$.

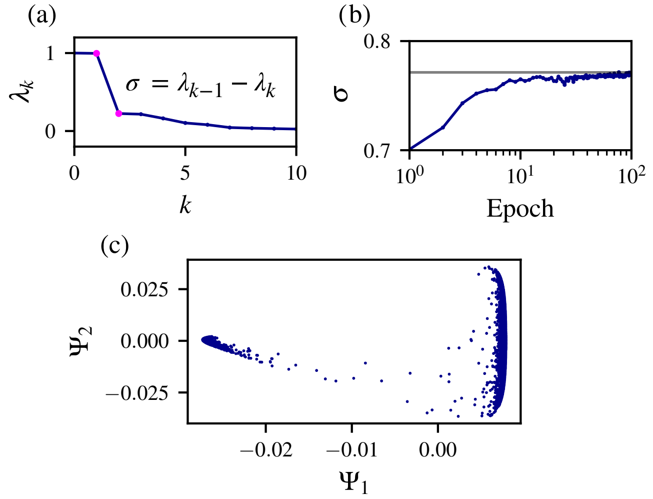


FIG. S2. Details of training the target mapping $\xi_w(\mathbf{x})$ for CLN025. (a) The spectrum of eigenvalues $\{\lambda_k\}$ calculated after the training from the complete data set of CV samples, showing a spectral gap of around 0.77. (b) Convergence of the spectral gap $\sigma$ during the training performed through 100 epochs. Spectral map values estimated batch-wise during the training converge to the spectral gap of the complete data set of CV samples. (c) Folded and unfolded states of CLN025 spanned by eigenvectors $\Psi_1$ and $\Psi_2$.

## S3. Markov State Model

We partition CV samples into 100 microstates, which are then used to perform an implied timescale analysis [Fig. S3(a) and Fig. S4]. For this, trial Markov probability matrices are created by counting the number of transitions between the microstates within a time lag $\tau$. We test time lags up to around 400 ns and observe that the dominant timescale does not depend on the lag time starting from around 100 ns [Fig. S3(b)] and thus, select the lag time of $\tau = 100$ ns for the construction of the Markov state model. The other timescales characteristic for the folding of chignolin are below the lag time, indicated by the grey area in Fig. S3(b) and not considered in the analysis. Based on the fact that there is only one important timescale, we assign each microstate to coarser macrostates by performing the Perron cluster-cluster analysis. The macrostates for the folded and unfolded metastable states are shown in Fig. S3(c). Next, we perform the Chapman–Kolmogorov test up to 1 $\mu$s to check the validity of our model and conclude that the Markov state model is constructed accurately, with very small error margins [Fig. S3(d)]. Based on this, we estimate mean first passage times to be $t_{\mathrm{F}} = 0.58 \pm 0.01$ $\mu$s for the transition between the unfolded and folded states and $t_{\mathrm{U}} = 2.08 \pm 0.02$ $\mu$s in the reverse direction.

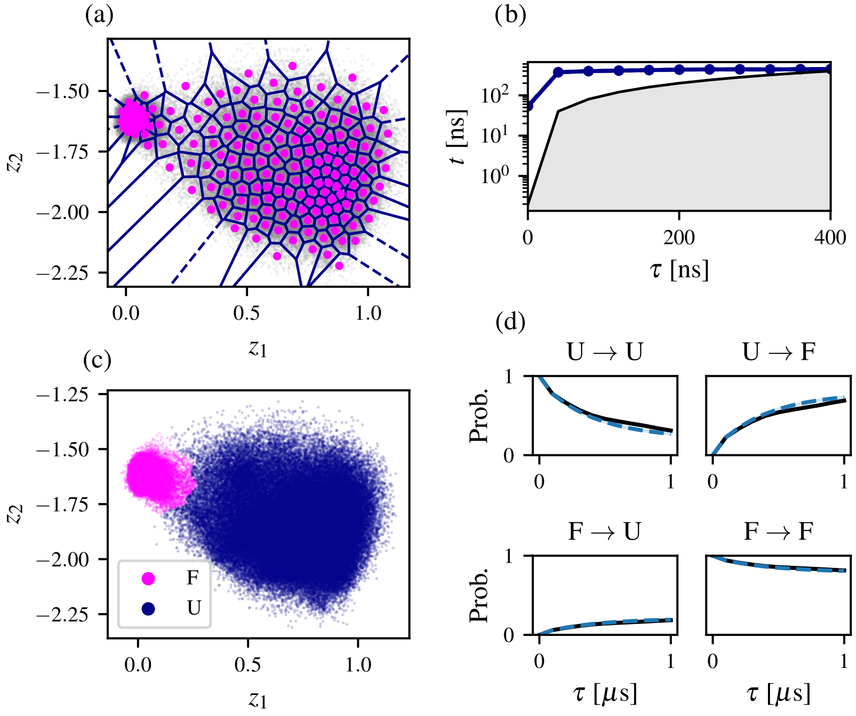


FIG. S3. Markov state model created from the CVs learned by spectral map applied to CLN025. (a) CV space is partitioned into 100 microstates (centers marked in magenta) using the $k$-means algorithm. (b) Implied timescale test performed to estimate the lag time $\tau = 100$ ns used to build a Markov state model and estimate the longest timescale (other timescales are lower than the lag time indicated by the grey area). (c) Assignment of the microstates into macrostates performed using the Perron cluster-cluster analysis. The folded state is colored in magenta, and the unfolded in blue. (d) Chapman–Kolmogorov test performed to validate the Markov state model, with transition probabilities between the folded and unfolded states.

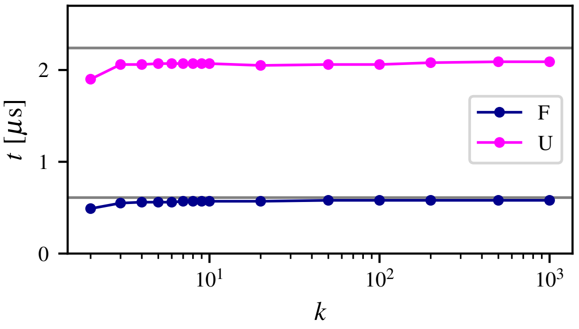


FIG. S4. Dependence of estimated mean times of the folding (F) and unfolding (U) of CLN025 on the number of clusters $k$ for the $k$-means algorithm. Reference values (shown in grey) are taken from Ref. 2.

## REFERENCES


[1] L. Bonati, E. Trizio, A. Rizzi, and M. Parrinello, "A Unified Framework for Machine Learning Collective Variables for Enhanced Sampling Simulations: `mlcolvar`," J. Chem. Phys. **159**, 014801 (2023).

[2] K. Lindorff-Larsen, S. Piana, R. O. Dror, and D. E. Shaw, "How Fast-Folding Proteins Fold," Science **334**, 517–520 (2011).

[3] A. Paszke, S. Gross, F. Massa, A. Lerer, J. Bradbury, G. Chanan, T. Killeen, Z. Lin, N. Gimelshein, L. Antiga, *et al.*, "PyTorch: An Imperative Style, High-Performance Deep Learning Library," in *Advances in Neural Information Processing Systems*, Vol. 32 (MIT Press, 2019) pp. 8026–8037.

[4] M. K. Scherer, B. Trendelkamp-Schroer, F. Paul, G. Pérez-Hernández, M. Hoffmann, N. Plattner, C. Wehmeyer, J.-H. Prinz, and F. Noé, "PyEMMA 2: A Software Package for Estimation, Validation, and Analysis of Markov Models," J. Chem. Theory Comput. **11**, 5525–5542 (2015).
